# Supplementary material for: Graphene-based electron transport layers in perovskite solar cells: a step-up for an efficient carrier collection
Source: arXiv:1702.04159 ancillary file (2017-05-16)
Supplement: Supplementary file 1 [file Supporting_Information.pdf]

# Supporting Information

## Material Characterization

The exfoliation of bulk graphite by liquid phase exfoliation (LPE) in N-methyl-2-pyrrolidone (NMP) gives a broad distribution of graphitic flakes, making a purification step necessary. We exploit sedimentation-based separation (SBS) to sort graphitic flakes by lateral size and thickness,[1] leaving the larger/thicker as well as un-exfoliated flakes at the bottom of the centrifuge tube, while the smaller/thinner flakes remain as supernatant. The concentration of the graphitic flakes in dispersion is calculated from the optical absorption spectroscopy (OAS) (Fig. 1), exploiting the optical absorption coefficient at 660nm ($\varepsilon_{660}$) of 1390 L $g^{-1}m^{-1}$,[2] giving a concentration of 0.25 g $L^{-1}$. The peak at ~266 nm in the spectrum is the signature of the van Hove singularity in the graphene density of states.[3]

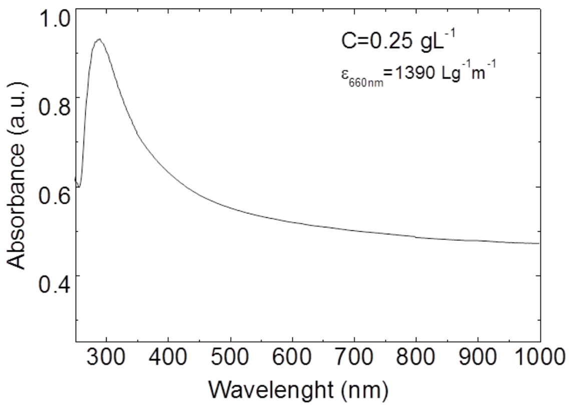


**Fig S1**. Optical absorption spectra of the graphene ink

The morphology of the flakes, *i.e.*, lateral size and thicknesses are characterized by transmission electron microscopy (TEM) and atomic force microscopy (AFM) respectively (see Fig. S2). A representative TEM image is reported (Fig 2a), and the statistical lateral size distribution, showing that the maximum population is centred at ~150 nm (Fig. 2b). The sample (Fig. 2c) contains flakes with an average thickness of 1.7 nm. The statistical analysis of the samples is shown in Figure 2d. Both distribution (lateral size and thickness) show the characteristic Log-normal distribution of fragmented systems in accordance with previous studies.[1,4]

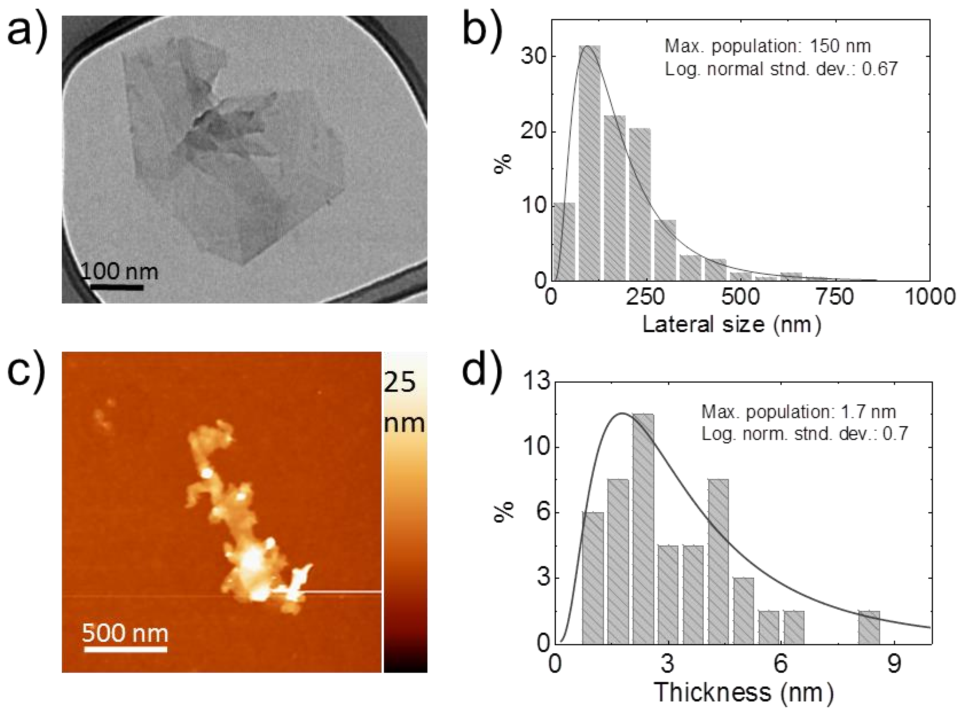


**Fig S2.** Size analysis of the graphene ink flakes. (a) Transmission electron micrograph of graphene flakes and (b) the statistical lateral size analysis. c) Atomic force microscopy of graphene flakes, and (d) the corresponding statistical thickness distribution.

The Raman spectrum of the graphene ink and graphite is shown for comparison in the Figure S3a. The Raman spectrum of the graphene flakes consists mainly in the G peak (~1580 $cm^{-1}$), originated from the $E_{2g}$ phonon mode at the Brillouin zone centre.[5] The D peak (~1347 $cm^{-1}$) corresponds to the breathing modes of $sp^2$ carbon rings, requiring a symmetry breaking for its activation.[6] The 2D peak is the second order of the D peak, appearing as a single peak for single layer graphene and as the superposition of multiple components for few-(FLG) and multi-layer graphene (MLG) flakes.[7] This peak does not require the presence of defects for its activation. The statistical Raman analysis gives information on the quality of the exfoliated graphitic flakes.[8,9] In particular, the 2D peak of the exfoliated samples is positioned, *i.e.*, Pos(2D) at ~2700 $cm^{-1}$ (Figure S3b), with its full wave at half maximum (*i.e.*, FWHM(2D)) that varies from 65 to 74 $cm^{-1}$ with a peak at ~67 $cm^{-1}$ (Figure S3c). The intensity ratio between the 2D and the G peak (I(2D)/I(G)) varies from 0.50 to 0.65 (Figure S3d). This suggests that the sample is composed by a combination of single layer graphene (SLG) and FLG flakes. The Raman spectrum of the graphene-based ink show significant D peak intensity, with an average intensity ratio I(D)/I(G) ~0.45 (Figure S3e). This is attributed to the edges of our nanometer flakes, rather than to the presence of structural defects on the basal plane of SLG and FLG flakes.[6] This observation is supported by the analysis of I(D)/I(G) (Figure S3e), FWHM(G) (Figure S3f) and Pos(G) (Figure S3g). Indeed, combining I(D)/I(G) with FWHM(G) allows us to discriminate between disorder localized at the edges and disorder in the bulk. In the latter case, a higher I(D)/I(G) would correspond to higher FWHM(G). The I(D)/I(G) and FWHM(G) of our sample are not correlated, as shown Figure S3h, which is a clear indication that the major contribution to the D peak comes from the sample edges.[1,8,9]

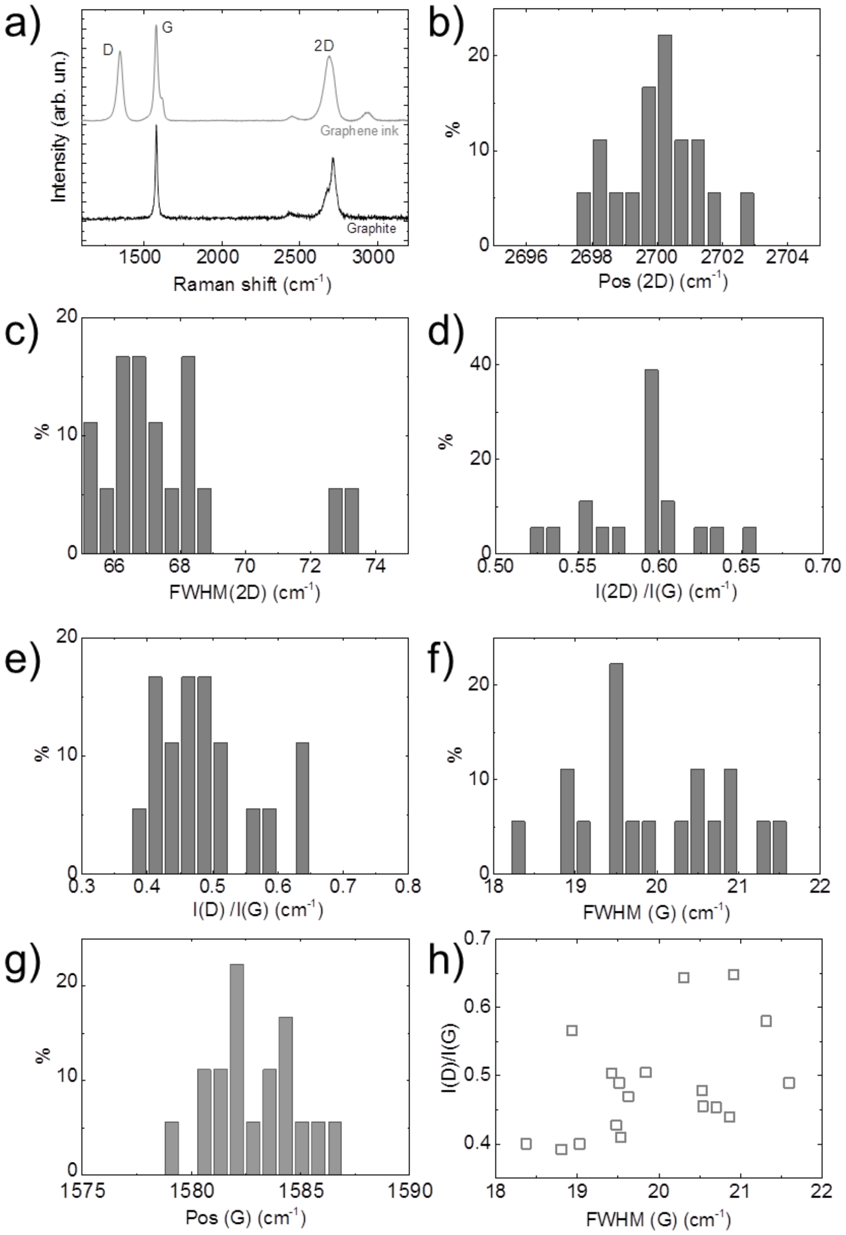


**Fig. S3**. a) Raman spectra of the exfoliated sample (in grey) and graphite (in black) for comparison. The Raman statistical analysis of the Pos(2D) (b), FWHM(2D) (c), I(2D)/I(G) (d), I(D)/I(G) (e), FWHM(G) (f), Pos(G) (g), and FWHM (G) vs I(D)/I(G).

## Photo-electrodes Characterization

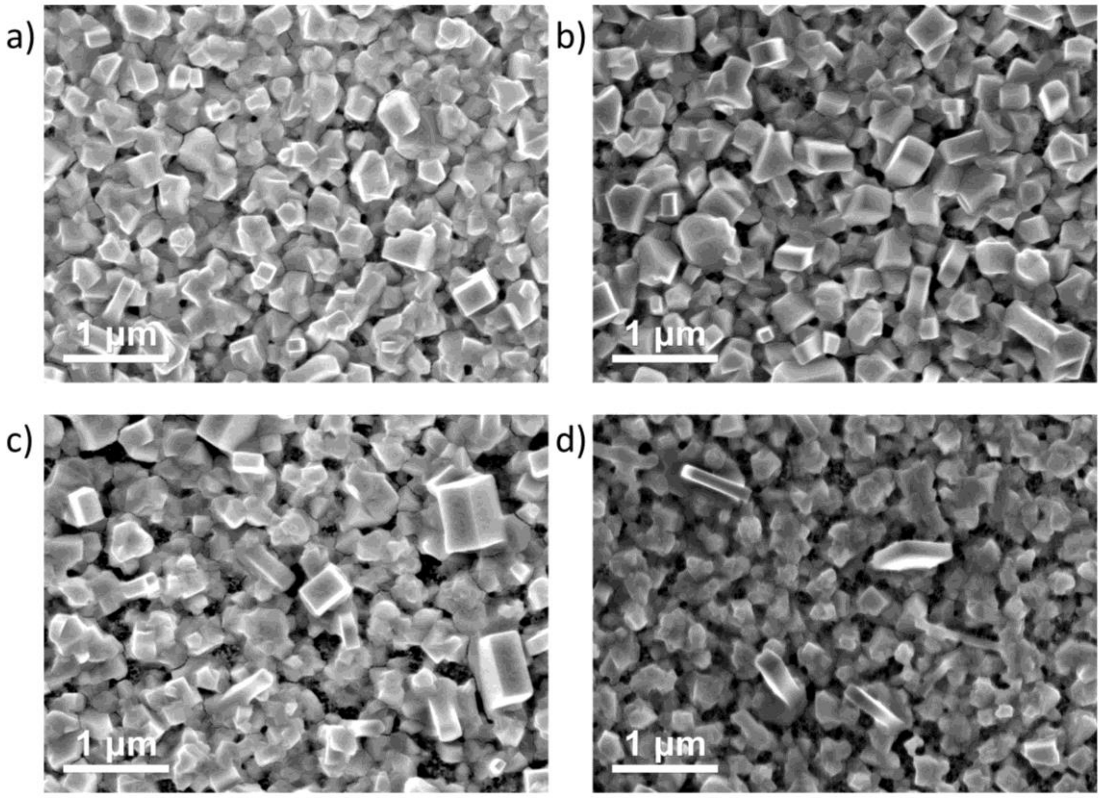


**Fig. S4** Scanning electron microscopy of the perovskite surface of different samples: a) ETL1, $mTiO_2$; b) ETL2, G+$mTiO_2$; c) ETL3, $mTiO_2$/GO-Li; d) ETL4, G+$mTiO_2$/GO-Li

All samples show typical cubic (tetragonal) perovskite crystals. Notably the crystal size and shape regularity seems to be enhanced by both the addition of graphene in the $mTiO_2$ layer and the interposition of a graphene oxide – Li electron transport layer.

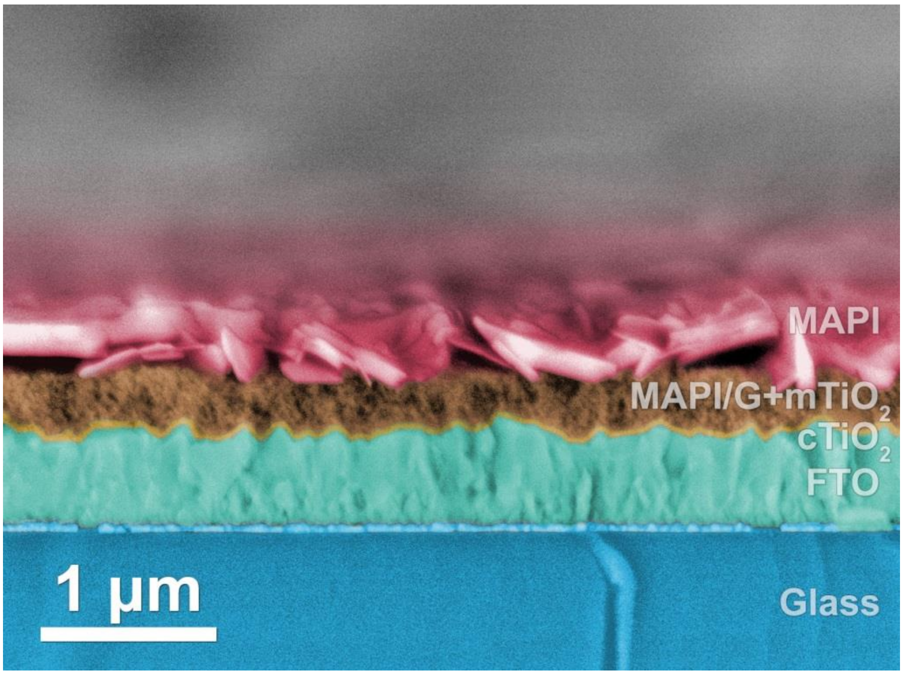


**Fig. S5**. Typical cross section of ETL2, G+m$TiO_2$, based cell.

In Fig.S5 it can be possible to determine the different layers constituting the device, *i.e.*, the FTO glass, the thin c$TiO_2$, the graphene + mTiO layer, the compenetration between perovskite and G+mTiO, with the perovskite crystals atop.

## Devices Characterization

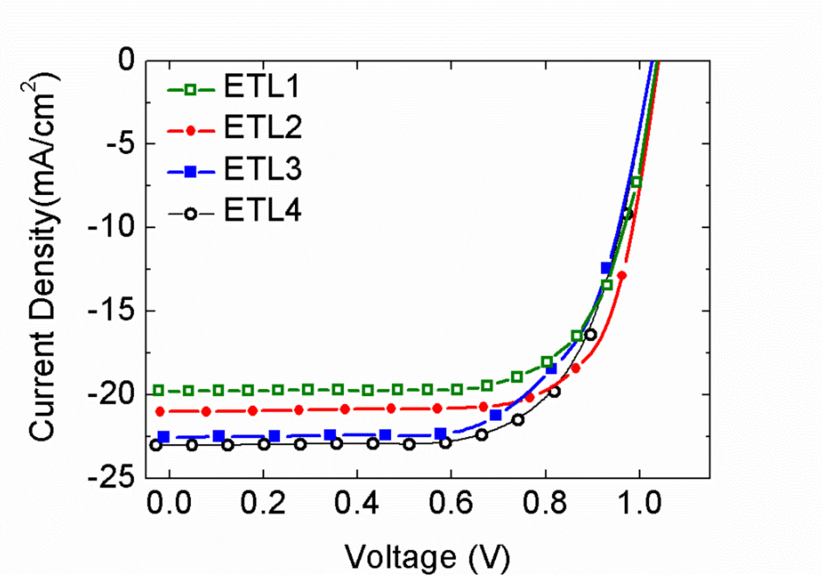


**Fig. S6**. Current Density-Voltage (J-V) characteristics of tested devices employing different ETLs (ETL1: m$TiO_2$, ETL2: m$TiO_2$/GO-Li, ETL3: G+m$TiO_2$, ETL4: m$TiO_2$/GO-Li).

| PE type | $V_{OC}$ (V) | $J_{SC}$ (mA/cm$^2$) | FF (%) | PCE (%) | Av. PCE (%) |
|---|---|---|---|---|---|
| ETL1: Ref | 1.038 | -19.74 | 71.4 | 14.6 | 13.00±0.30 |
| ETL2: G+m$TiO_2$ | 1.041 | -20.99 | 73.2 | 16.0 | 14.20±0.39 |
| ETL3: GO-Li | 1.029 | -22.51 | 65.5 | 15.2 | 14.13±0.30% |
| ETL4: G+m$TiO_2$/GO-Li | 1.031 | -22.85 | 68.9 | 16.2 | 14.72±0.24% |

**Tab. S1**. Electrical parameters (open-circuit voltage, $V_{OC}$; short-circuit current density, $J_{SC}$; fill factor, FF; and power conversion efficiency, PCE) of the best performing devices for each tested photo-electrodes (ETL1: m$TiO_2$, ETL2: m$TiO_2$/GO-Li, ETL3: G+m$TiO_2$, ETL4: m$TiO_2$/GO-Li). The last column reports the average efficiency calculated on 10 devices.

The J-V characteristics reported in Fig. S6 show a remarkable improvement in power conversion efficiency (PCE) when graphene-based ETLs are employed in complete devices. In particular, the best performing device based on ETL4 (G+m$TiO_2$/GO-Li) exhibits PCE overcoming 16% with a considerable increase in short circuit current density ($J_{SC}$). Moreover, the standard error calculated on 10 devices is considerably reduced in the case of ETL4.

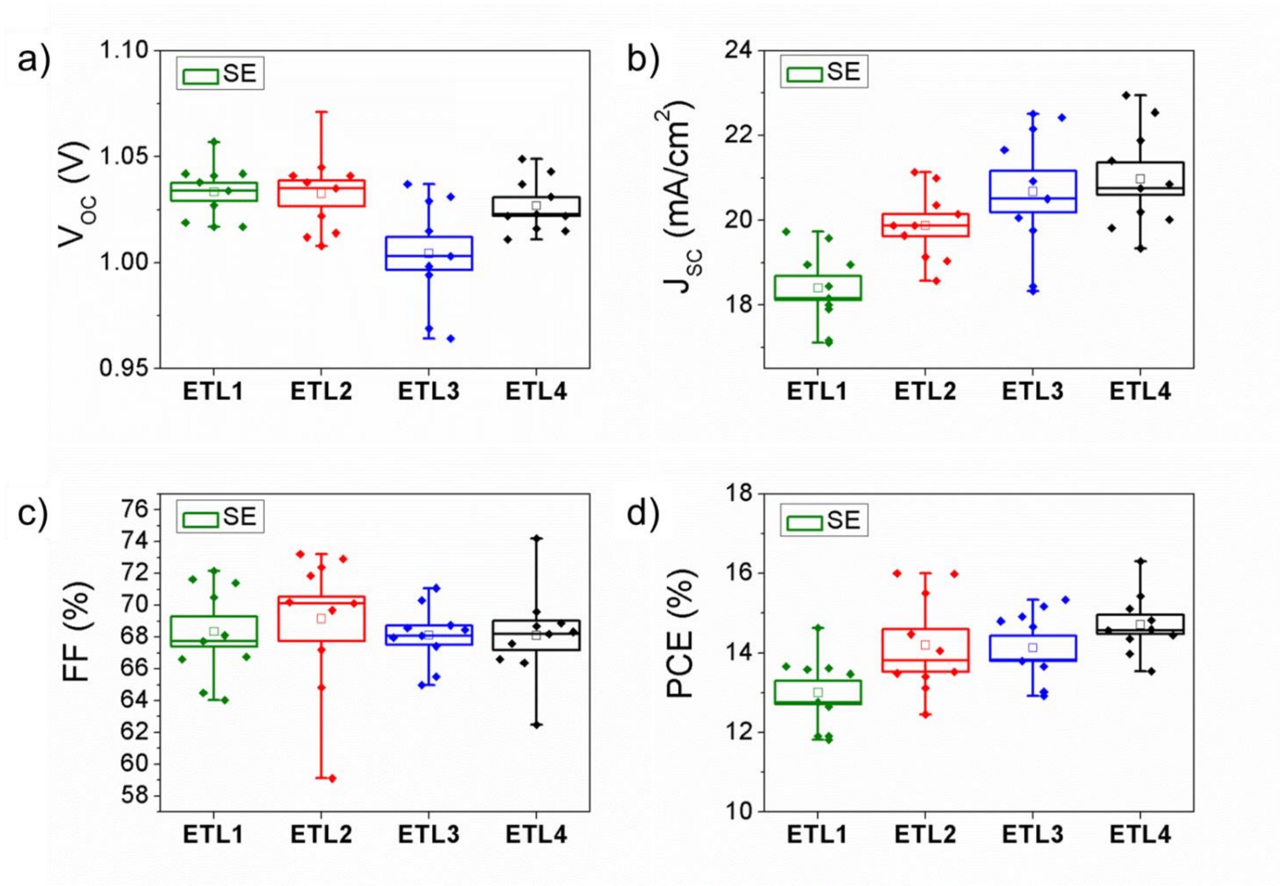


**Fig. S7**. Photovoltaic parameters measured at 1 SUN and relative standard error (SE) on 10 cells (open-circuit voltage, $V_{OC}$; short-circuit current density, $J_{SC}$; fill factor, FF; and power conversion efficiency, PCE reported in panels a, b, c, and d, respectively), for the four investigated ETLs. (ETL1: m$TiO_2$, ETL2: m$TiO_2$/GO-Li, ETL3: G+m$TiO_2$, ETL4: m$TiO_2$/GO-Li).

The statistics on 10 samples for each tested ETL are reported in Fig.S7 considering the electrical parameters extracted by the 1 SUN J-V curves. Notably $J_{SC}$ is remarkably increased when graphene-based ETLs are employed, due to an improved charge transfer from perovskite to the ETL.

**References**


[1] G. Kakavelakis, A. E. Del Rio Castillo, V. Pellegrini, A. Ansaldo, P. Tzourmpakis, R.Brescia, M. Prato , E. Stratakis, E. Kymakis , and F. Bonaccorso, Size-Tuning of WSe2 Flakes for High Efficiency Inverted Organic Solar Cells, ACSnano, 2017, 10.1021/acsnano.7b00323

[2] M. Lotya, Y. Hernandez, P. J. King, R. J. Smith, V. Nicolosi, L. S. Karlsson, F. M. Blighe, S. De, W. Zhiming, I. T. McGovern, G. S. Duesberg, J. N. Coleman, J. Am. Chem. Soc. 2009, 131, 3611.

[3] V. G. Kravets, A. N. Grigorenko, R. R. Nair, P. Blake, S. Anissimova, K. S. Novoselov and A. K. Geim, Phys. Rev. B - Condens. Matter Mater. Phys., 2010, 81, 1–6

[4] Kouroupis-Agalou K, Liscio A, Treossi E, Ortolani L, Morandi V, Pugno NM, Palermo V, Nanoscale, Fragmentation and exfoliation of 2D Materials. A statistical approach, (2014) 6, 5926-5933

[5] A. Ferrari and D. Basko, Nat. Nanotechnol., 2013, 8, 235–46.

[6] A. C. Ferrari and J. Robertson, Phys. Rev. B, 2001, 64, 1–13

[7] A. C. Ferrari, J. C. Meyer, V. Scardaci, C. Casiraghi, M. Lazzeri, F. Mauri, S. Piscanec, D. Jiang, K. S. Novoselov, S. Roth and A. K. Geim, Phys. Rev. Lett., 2006, 97, 187401–187405.

[8] A. Capasso, A. E. Del Rio Castillo, H. Sun, A. Ansaldo, V. Pellegrini and F. Bonaccorso, Solid State Commun., 2015, 224, 53–63

[9] F. Torrisi, T. Hasan, W. Wu, Z. Sun, A. Lombardo, T. S. Kulmala, G.-W. Hsieh, S. Jung, F. Bonaccorso, P. J. Paul, D. Chu and A. C. Ferrari, ACS Nano, 2012, 6, 2992–3006.
